# Supplementary material for: On Logics and Homomorphism Closure
Source: arXiv:2104.11955 source file (2021-06-29)
Supplement: Supplementary file 1 [file appendix-lost-and-found.tex]

\subsection{Everything about the Projective Characterization Cases}

\bigskip

\probbox{
	\textbf{Problem:} $\mathrm{InProjHomCl}_\mathrm{(fin)}$\\
	\textbf{Input:} $\tau$, $\tau'$ with $\tau\subseteq\tau'$, sentence $\Phi$ over $\tau'$, finite $\tau$-structure $\mathfrak{A}$.\\
	\textbf{Output:} \textsc{yes}, if $\mathfrak{A} \in \homcl{\getffinmodels{\Phi}|_\tau}$, \textsc{no} otherwise.  
}

\bigskip

\begin{proposition}
	$\mathrm{InHomCl}$ and $\mathrm{InProjHomCl}$ are \textsc{LogSpace}-interreducible, and so are 
	$\mathrm{InHomCl}_\mathrm{fin}$ and $\mathrm{InProjHomCl}_\mathrm{fin}$.
\end{proposition}

\begin{proof}
	$\mathrm{InHomCl}_\mathrm{(fin)} \Rightarrow \mathrm{InProjHomCl}_\mathrm{(fin)}$: special case, pick $\tau=\tau'$.
	
	$\mathrm{InProjHomCl}_\mathrm{(fin)} \Rightarrow \mathrm{InHomCl}_\mathrm{(fin)}$: let $\sigma = \tau'\setminus \tau$. Then $\mathrm{InProjHomCl}_\mathrm{(fin)}$ holds for $\Phi$ and $\mathfrak{A}$ exactly if $\mathrm{InHomCl}_\mathrm{(fin)}$ holds for $\Phi$ and $\mathfrak{A}\cdot \widehat\sigma$.
\end{proof}

We conclude this section by briefly looking at the projective characterization variant of the homclosedness problem.

\bigskip

\probbox{
	\textbf{Problem:} $\mathrm{ProjHomClosed}_\mathrm{(fin)}$\\
	\textbf{Input:} $\tau$, $\tau'$ with $\tau\subseteq\tau'$, sentence $\Phi$ over $\tau'$.\\
	\textbf{Output:} \textsc{yes}, if $\getffinmodels{\Phi}|_\tau = \homclffin{\getffinmodels{\Phi}|_\tau}$, \textsc{no} otherwise.  
}

\bigskip

As it turns out, the situation becomes pretty hopeless there; the problem turns undecidable already for very inexpressive logics,
since they allow for projectively characterizing $\neg(\Phi_{\mathcal{D}\text{-}\mathrm{tiling}} \wedge \neg\exists x.\sigT{}_\emptyset{}(x))$.

\begin{theorem}[restate=hopeless, name=]
	$\mathrm{ProjHomClosed}_\mathrm{(fin)}$ is undecidable even for 
	\begin{enumerate}[itemindent=0ex, leftmargin=3ex, itemsep=-0.5ex]
		\item 
		$\Al\FO$ with predicate arity $\leq 2$ and three constants,
		\item 
		$\FOt$ without constants, and
		\item
		$\mathbb{GFO}$ without constants and with maximum arity $\leq 3$.
	\end{enumerate} 
\end{theorem}

\begin{proof}
	\begin{enumerate}[itemindent=0ex, leftmargin=3ex, itemsep=-0.5ex]
		\item 
		Take $\neg\Phi_{\mathcal{D}\text{-}\mathrm{tiling}} \vee \exists x.\sigT{}_\emptyset{}(x)$, put it in prenex (carefully reusing variables where possible), skolemize leading existential quantifiers into constants. Choose $\tau$ such that the constants are removed. 
		\item
		As before but ``paraphrase'' the three constants by unary predicates, axiomatized to be nonempty. Then choose $\tau$ such that the unary predicates are removed.
		\item
		Take  $\neg\Phi_{\mathcal{D}\text{-}\mathrm{tiling}} \vee \exists x.\sigT{}_\emptyset{}(x)$, put it in NNF. The obtained sentence is almost guarded, except for the subsentence with prefix $\exists xyz ...$, which we replace by $\exists xyz. \sig{Ter}(x,y,z) \wedge ...$ where $\sig{Ter}$ is a fresh ternary predicate. Then choose $\tau$ such that $\sig{Ter}$ is removed again.\qedhere
	\end{enumerate} 
\end{proof}

\subsection{lost and found -- probably not longer needed}

\begin{definition}\label{def:TGDdettiling}
	Given a deterministic domino system
	$\mathcal{D}=(D,B,L,\sigH{},\sigV{})$, let $$\Phi_{\mathcal{D}\text{-}\mathrm{tiling}} = \forall xyz. \exists v. \Phi_\mathcal{D}$$ where $\Phi_\mathcal{D}$ is the conjunction over the following rules (introducing unary predicates $\sigT{}_\emptyset$ and $\sigT{}_{\{d\}}$ for all the dominoes $d \in D_\mathcal{D}$):
	\begin{eqnarray}
		& \!\!\!\!\to\!\!\!\! & Eq(x,x) \\
		Eq(x,y) \wedge Eq(y,z)  & \!\!\!\!\to\!\!\!\! & \sigH{}(x,v) \\
		\sigH{}(x,y) \wedge Eq(y,z)  & \!\!\!\!\to\!\!\!\! & \sigV{}(x,v) \\
		\sigV{}(x,y) \wedge Eq(y,z)  & \!\!\!\!\to\!\!\!\! & \sigT{}_{B \cap L}(v) \\
		\sigH{}(x,y) \wedge \sigV{}(x,z) & \!\!\!\!\to\!\!\!\! & \sigH{}(z,v) \wedge \sigV{}(y,v)\\[2ex]
		\sigT{}_{\{d\}}(x) \wedge \sigV{}(x,y) & \!\!\!\!\to\!\!\!\! & \sigT{}_{\sigV{}(d)}(y) \\
		\sigT{}_{\{d\}}(x) \wedge \sigH{}(x,y) & \!\!\!\!\to\!\!\!\! & \sigT{}_{\sigH{}(d)}(y) \\
		\sigT{}_{\{d_1\}}(x) \wedge \sigH{}(x,z) \wedge \ \  \nonumber \\[-3pt]
		\sigT{}_{\{d_2\}}(y) \wedge \sigV{}(y,z) & \!\!\!\!\to\!\!\!\! & 
		\sigT{}_{\sigH{}(d_1)\cap \sigV{}(d_2)}(y) \\
		\sigT{}_{\{d_1\}}(x) \wedge \sigT{}_{\{d_2\}}(x) & \!\!\!\!\to\!\!\!\! &
		\sigT{}_{\{d_1\}\cap\{d_2\}}(x)
	\end{eqnarray}
\end{definition}

It is trivial to equivalently rewrite $\Phi_{\mathcal{D}\text{-}\mathrm{tiling}}$ into a \TGD{} sentence, so we will consider it as such, whenever convenient.

\begin{lemma}
	\begin{enumerate}
		\item
		$\Phi_{\mathcal{D}\text{-}\mathrm{tiling}}$ is a $\AAAE$ formula.
		\item
		Any -- finite or infinite -- model $\mathfrak{A}$ of $\Phi_{\mathcal{D}\text{-}\mathrm{tiling}}$ admits a homomorphism into and a homomorphism from $\mathfrak{A} \uplus \mathfrak{I}$, which is not a model of $\Phi_{\mathcal{D}\text{-}\mathrm{tiling}}$. 
		Moreover $\sigT{}_\emptyset{}^\mathfrak{A} = \sigT{}_\emptyset{}^{\mathfrak{A}\uplus \mathfrak{I}}$.
		\item
		$\Phi_{\mathcal{D}\text{-}\mathrm{tiling}}$ has a (finite) model $\mathfrak{A}$ with $\sigT{}_\emptyset{}^\mathfrak{A} = \emptyset$
		exactly if there is a (ultimately periodic) $\mathcal{D}$-tiling.
		\item
		$\Phi_{\mathcal{D}\text{-}\mathrm{tiling}}$ (finitely) entails the \CQ{} $\exists x.\sigT{}_\emptyset{}(x)$ exactly if there exists no
		(ultimately periodic) $\mathcal{D}$-tiling.
		\item 
		The class of (finite) models of the \MDTGD{} sentence $\Psi = \Phi_{\mathcal{D}\text{-}\mathrm{tiling}} \vee \exists x.\sigT{}_\emptyset{}(x)$ is closed under (finite-target) homomorphisms exactly if there exists no
		(ultimately periodic) $\mathcal{D}$-tiling. Moreover, $\Psi$ is a \MDTGD{} sentence and expressible as a $\AAAE$ sentence.
	\end{enumerate}
\end{lemma}

\begin{corollary}
	$\mathrm{\sigH{}omClosed}_\mathrm{(fin)}$ is undecidable for \MDTGD{} (and hence for \DTGD{}).
	This even holds for \DTGD{} sentences wherein every rule uses only unary and binary predicates as well as $\leq$3 universally and $\leq$1 existentially quantified variables. 
\end{corollary}

We will put to use the previously introduced machinery for a few more undecidability results.

\begin{lemma}
	$\neg\Phi_{\mathcal{D}\text{-}\mathrm{tiling}} \vee \exists x.\sigT{}_\emptyset{}(x)$
	\begin{enumerate}
		\item
		is equivalent to a \EEEA{} sentence with all predicates of arity $\leq 2$,
		\item
		is (finitely) valid exactly if there is no (ultimately periodic) $\mathcal{D}$-tiling, and
		\item
		has a (finite) model class closed under (finite-target) homomorphisms exactly if it is (finitely) valid.
	\end{enumerate}
\end{lemma}

This directly entails the following theorem establishing undecidability for a $\FOe$ fragment whose satisfiability problem is decidable (and, in fact, even in \textsc{NP}).

\begin{theorem}
	$\mathrm{\sigH{}omClosed}_\mathrm{(fin)}$ is undecidable for $\Ex\Ex\Ex\Al\FO$ even with predicates of arity $\leq 2$ and with no constants.
\end{theorem}

\subsection{Another Lost-and-Found: Open Prefix Classes (mostly fragments, really)}

With the above results established, the remaining prefix classes where decidability of $\mathrm{\sigH{}omClosed}_\mathrm{(fin)}$ is still open are $\AEEE$, $\EAAA$, $\AEEe$, and $\EAAe$.

We now turn to $\AEEE$ 

\begin{definition} Let $\mathcal{D}=(D,D,D,H,V)$ be a classical domino system.
	Let $\Phi^{\forall\exists\exists}_\mathcal{D}$ denote the $\AEEE$ sentence $\forall x \exists yz. Exc(x) \vee (\sigH{}(x,y) \wedge \sigV{}(x,z))$.
	Let $\Phi^{\forall\forall\forall}_\mathcal{D}$ denote the $\EAAA$ sentence $\forall xyz. \Psi$ where $\Psi$ is the conjunction over the following formulae:
	
	%\noindent $E(x,x)$ \hfill $E(x,y) \,{\to}\, E(y,x)$ \hfill $E(x,y)\, {\wedge}\,  E(y,z)\,  {\to}\,  E(x,z)$\\
	%\noindent $E(x,y) \, {\wedge}\,  \sigH{}(x,z) \, {\to}\,  \sigH{}(y,z)$ \hfill $E(y,z) \, {\wedge}\,  \sigH{}(x,y) \, {\to}\,  \sigH{}(x,z)$\\
	%\noindent $E(x,y) \, {\wedge}\,  \sigV{}(x,z) \, {\to}\,  \sigV{}(y,z)$ \hfill $E(y,z) \, {\wedge}\,  \sigV{}(x,y) \, {\to}\,  \sigV{}(x,z)$\\[1ex]
	\noindent $\sigH{}(x,y) \, {\wedge}\,  \sigV{}(x,z) \, {\to}\, \sigH{}\sigV{}(y,z)$ \hfill $\sigH{}\sigV{}(x,y) \, {\wedge}\,  \sigV{}(y,z) \, {\to}\, \sigH{}(x,z)$\\
	\noindent $\sigH{}(x,y)\, {\to}\, \bigvee_{(d,d')\in \sigH{}} \sigT{}_{\{d\}}(x) \wedge \sigT{}_{\{d'\}}(y)$ \\
	\noindent $\sigV{}(x,y)\, {\to}\, \bigvee_{(d,d')\in \sigV{}} \sigT{}_{\{d\}}(x) \wedge \sigT{}_{\{d'\}}(y)$ \\
	\noindent $\sigT{}_{\{d\}}(x) \wedge \sigT{}_{\{d'\}}(x)\, {\to}\, \sigT{}_{\{d\}\cap \{d'\}}(x)$ \\
	\noindent $Exc(x) \to \bot$\\
	\noindent $\neg \sigT{}_{\emptyset}(x)$\\
	
	Moreover, for every $P \in \{\sigH{},\sigV{},\sigH{}\sigV{},Exc,\sigT{}_S\}$ we add $\neg P(\bold{x}) \leftrightarrow \overline{P}(\bold{x})$ as well as $\overline{P}(\bold{x}) \wedge P(\bold{x}) \to \bot$.

\end{definition}

\newcommand{\formula}{\Phi^{\forall\exists\exists}_\mathcal{D}\! \wedge \!\!\, \neg \Phi^{\forall\forall\forall}_\mathcal{D}}

\begin{lemma}
	\begin{enumerate}
		\item
		$\Phi^{\forall\exists\exists}_\mathcal{D} \wedge \Phi^{\forall\forall\forall}_\mathcal{D}$ is (finitely) satisfiable exactly if there exists a (ultimately periodic) $\mathcal{D}$-tiling.
		\item
		$\Phi^{\forall\exists\exists}_\mathcal{D}$ (finitely) entails $\neg \Phi^{\forall\forall\forall}_\mathcal{D}$ exactly if there exists no (ultimately periodic) $\mathcal{D}$-tiling.
		\item
		????$\formula$
		is finitely equivalent to $\neg \Phi^{\forall\forall\forall}_\mathcal{D}$ exactly if there exists no (ultimately periodic) $\mathcal{D}$-tiling.
		\item 
		A (finite) spoiler of $\formula$ exists exactly if there exists a (ultimately periodic) $\mathcal{D}$-tiling.
	\end{enumerate}
\end{lemma}

\begin{proof}
	...
	
	Let $\mathfrak{A}\stackrel{h}{\to}\mathfrak{B}$ be a (finite) spoiler for $\formula$. Due to the absence of equality in our logic and thanks to Corollary~\ref{lem:inj-or-ss}, we can without loss of generality assume that $h$ is injective. By definition 
	$\mathfrak{A} \in \getffinmodels{\formula}$ but $\mathfrak{B} \not\in \getffinmodels{\formula}$.
	In particular this means that $\mathfrak{B} \in \getffinmodels{\neg \Phi^{\forall\exists\exists}_\mathcal{D}}$ or $\mathfrak{B} \in \getffinmodels{\Phi^{\forall\forall\forall}_\mathcal{D}}$. 
	
	We proceed by case distinction: assume $\mathfrak{B} \in \getffinmodels{\neg \Phi^{\forall\exists\exists}_\mathcal{D}}$. Then, there must be some $b \in B$ with 
	$b \not\in Ex\sigc{}^\mathfrak{B}$ and ...

	Let now $B' = h(A)$ and let $\mathfrak{B}'$ denote the $B'$-induced substructure of $\mathfrak{B}$. Then $h:\mathfrak{A} \to \mathfrak{B}'$ is a surjective homomorphism, hence a bijection (since injectivity was already established above). As surjective homomorphisms preserve positive formulae, it follows that $\mathfrak{B}'\models \Phi^{\forall\exists\exists}_\mathcal{D}$. 
	
	We proceed by case distinction as to whether $\mathfrak{B}'\models \Phi^{\forall\forall\forall}_\mathcal{D}$:
	
	Assume $\mathfrak{B}'\models \neg\Phi^{\forall\forall\forall}_\mathcal{D}$.
	But then $\mathfrak{B'}\stackrel{id_{B'}}{\to}\mathfrak{B}$ is an embedding spoiler.

	$\mathfrak{B} \in \getffinmodels{\neg \Phi^{\forall\exists\exists}_\mathcal{D}}$:
	This means there must be some

	Since $\Phi^{\forall\forall\forall}_\mathcal{D}$ is purely universal, this implies 
	$\mathfrak{B}' \in \getffinmodels{\Phi^{\forall\forall\forall}_\mathcal{D}}$ and $h:\mathfrak{A} \to \mathfrak{B}'$ is a surjective homomorphism, hence a bijection (since injectivity was already established above).

	Moreover it is necessarily strong: the signature contains complement predicates, which are axiomatized such that $P^{\mathfrak{B}'} = B' \setminus \overline{P}^{\mathfrak{B}'}$. Thus assuming  
	
	Surjective homomorphisms preserve positive sentences (i.e. sentences with arbitrary quantifiers but only the connectives $\wedge$ and $\vee$) (CITE SOME MODEL THEORY BOOK?)

\end{proof}

With $\mathrm{HomClosed}_\mathrm{(fin)}$ shown to be undecidable for $\AAAE$ and $\EEEA$ as well as $\AAEe$ and $\EEAe$, the remaining maximal prefix classes (having a decidable satisfiability problem) are $\EsFO$, $\AsFO$, $\AAEE$, $\EEAA$, $\AEEe$, and $\EAAe$.

\appendix{Looks like we don't need non-squashing homs after all -- so I put them here}

\begin{definition}
	A homomorphism $h: \mathfrak{A} \to \mathfrak{B}$ is called \emph{non-squashing} if $B$ is infinite or $|A| \leq |B|$. 	
\end{definition}

In particular any injective homomorphism is \emph{non-squashing}.

\begin{definition}
	Let $\Phi$ be an arbitrary $\ESO$ sentence over signature $\tau$ with first-order part $\Psi$ over signature $\sigma \supseteq \tau$. We let $\tau'$ be the signature containing fresh copies $\sigP{}'$ and $\sigc{}'$ for all predicates $\sigP{}$ and constants $\sigc{}$, respectively, from $\tau$. Let $\Psi_{\tau \mapsto \tau'}$ denote the $\FOe$ sentence over $\tau' \cup \sigma \setminus \tau$ obtained by replacing in $\Psi$ all occurrences of signature elements from $\tau$ by their respective counterparts from $\tau'$.    
	
	Let now $$\Phi^\mathrm{ns} =  \Psi_{\tau \mapsto \tau'}^{\mathrm{rel}(\sigU{})} \wedge \Psi_\mathrm{HomAx}$$
	where $\Psi_\mathrm{HomAx}$ is the conjunction over the following sentences (introducing a fresh binary predicate $\sigF{}$):
	\begin{eqnarray}
		\forall x. \sigU{}(x) & \!\!\!\!\impl\!\!\!\! & \exists y. \sigF{}(x,y)\ \ \ \ \ \ \  \\
		\forall xyz. \sigF{}(x,y) \wedge \sigF{}(x,z) & \!\!\!\!\impl\!\!\!\! & y = z \\
		\bigwedge_{{\sigc{}'\in \mathrm{const}(\tau')}} \sigF{}(\sigc{}',\sigc{}) & & \\
		\bigwedge_{{\sigP( \tau}\atop{k=\text{ar}(\sigP)}} \bigg( \forall \bold{x} \bold{y} \sigP{}'(\bold{x}) \wedge \big(\smallbigwedge_{i=1}^k \sigF{}(x_i,y_i)\big) 
		& \!\!\!\!\impl\!\!\!\! & \sig\sigP(\bold{y}) \bigg)
	\end{eqnarray}
	with $\bold{x} = x_1,\ldots,x_k$ and $\bold{y} = y_1,\ldots,y_k$. Finally, we let
	$$ \Phi_{\mathrm{char}}^\mathrm{ns} = \exists \sigU{}. \exists \sigF{}.\exists \tau' \cup \sigma \setminus \tau.\big(\Phi^\mathrm{ns}\big),$$
	where $\exists \tau' \cup \sigma \setminus \tau$ abbreviates the existential (second-order) quantification over predicates from $\tau' \cup \sigma \setminus \tau$ (now taking the role of second-order variables) followed by the existential (first-order) quantification over constants from $\tau' \cup \sigma \setminus \tau$ (now taking the role of first-order variables). 
\end{definition}

\begin{theorem}
	For any $\ESO{}$ sentence $\Phi$, the closure of $\getmodels{\Phi}$ under non-squashing homomorphisms is projectively characterized by by the $\FOe$ sentence $\Phi^\mathrm{ns}$ and characterized by the $\ESO$ sentence $\Phi_{\mathrm{char}}^\mathrm{ns}$.
\end{theorem}

\begin{proof}
	Not so difficult to see. The case where an uncountable model is mapped to a countable target structure requires to invoke Theorem~\ref{the:LoSk}.
\end{proof}

\appendix{Another Lost and Found – I don't think this is needed any more}

\subsection{Some Observations on Homomorphisms, $\FOe$, and  $\ESO$}

The following are straightforward consequences of the L\"owenheim-Skolem theorem.

\begin{theorem}\label{the:LoSk}
	For every countable $\ESO$ theory $\Xi$ holds $\homcl{\getmodels{\Xi}} = \homcl{\getctblmodels{\Xi}}$. 
	Moreover, for any two countable $\ESO$ theories $\Xi_1$ and $\Xi_2$ holds $$\homcl{\getmodels{\Xi_1}}=\homcl{\getmodels{\Xi_2}}\ \ \text{exactly if}\ \  \homclctbl{\getmodels{\Xi_1}}=\homclctbl{\getmodels{\Xi_2}}.$$  
\end{theorem}

In order to see that the second part of this theorem cannot be strengthened to finite-target homomorphisms (rather than countable-target ones), even when restricting to single $\FO$ sentences, consider $\Xi_1 = \{\forall xy. \sig\sigP(x,y) \impl \exists z \sig\sigP(y,z)\}$ and $\Xi_2 = \{\forall xy. \sig\sigP(x,y) \impl \exists zv. \sig\sigP(v,x) \wedge \sig\sigP(y,z)\}$. Note that $(\mathbb{N},\{(i,i+1)\})$ is a model of $\Xi_1$ but not of $\Xi_2$ (and also not contained in $\homcl{\getmodels{\Xi_2}}$), while $\homclfin{\getmodels{\Xi_1}}=\homclfin{\getmodels{\Xi_2}}$.
